# Supplementary material for: DumbleDR: Predicting User Preferences of Dimensionality Reduction Projection Quality
Source: arXiv:2105.09275 source file (2021-05-19)
Supplement: Supplementary file 1 [file appendix.tex]

\section{Supplementary Material: Quality Measure Equations}

$LCMC$ is defined as
\begin{equation}
    LCMC(k) = \frac{1}{n} \sum_{i=1}^{n} |\nu_{i}^{k} \cap \rho_{i}^{k}|,
\end{equation}
where $n$ is the number of points and $\nu_{i}^{k}$ (resp. $\rho_{i}^{k}$) is the set of the $k$ nearest neighbors of the point $i$ in the original data (resp. in the visualization). T\&C combines two measures. The first one is the trustfulness of the visualization for a neighborhood size $k$, which is defined by
\begin{equation}
    T(k) = 1 - \frac{2}{nk(2n - 3k - 1)} \sum^n_{i=1} \sum_{j \in U_k(i)} (r^{HD}(i, j) - k),
\end{equation}
where $r^{HD}(i, j)$ is the rank of the $j^{th}$ point in terms of distance to the point $i$ in the original data and $U_k(i)$ is the set of the $k$ nearest neighbors of point $i$ in the visualization that are not among the $k$ nearest neighbors of  point $i$ in the original data. This metric measures whether we can trust what can be seen in the visualization. The measure of continuity is the exact opposite, as it tells how well the patterns from the original dataset are projected in the visualization. The continuity for a particular neighborhood size $k$ is defined by
\begin{equation}
    C(k) = 1 - \frac{2}{nk(2n - 3k - 1)} \sum^n_{i=1} \sum_{j \in V_k(i)} (r^{LD}(i, j) - k), 
\end{equation}
where $r^{LD}(i, j)$ is the rank of the $j^{th}$ in terms of distance to the point $i$ in the visualization and $V_k(i)$ is the set of the $k$ nearest neighbors of point $i$ in the original data that are not among the $k$ nearest neighbors of point $i$ in the visualization.

% Not sure we have to talk about Q_y, we didn't implement it.
%Other metrics combine local neighborhood with global patterns (e.g. $Q_y$). 

While the previously mentioned approaches focus on a specific neighborhood size $k$, $AUC_{log}RNX$ consider all neighborhood sizes, with a focus on smaller neighborhoods. In order to do so, $AUC_{log}RNX$ considers the neighborhood sizes with a logarithmic importance:
\begin{equation}
AUC_{log}RNX =
    {\left(\sum_{k=1}^{n-2} \frac{R_{NX}(k)}{k} \right)} /
    {\left(\sum_{k=1}^{n-2}\frac{1}{k}\right)},
\end{equation}
where 
\begin{equation} 
R_{NX}(k) =  \frac{(n-1) Q_{NX}(k) - k}{n - 1 - k},
\end{equation}
and where 
\begin{equation}
Q_{NX}(k) = \frac{1}{nk} \sum_{i=1}^{n} |\nu_{i}^{k} \cap \rho_{i}^{k}|.
\end{equation}

The other community that tackles the measure of visualization quality is the visualization (VIS) community. This community developed well-known measures for the detection of patterns in  visualizations (e.g. Scagnostics measures~\cite{wilkinson2005,wilkinson2006}). These types of measures allow users to measure the sparsity in the visualization, the skewness or even the presence of outliers.

More recently, it has been shown that cluster separability measures can match user perception in visualizations~\cite{sedlmair2015quality}. In particular, distance consistency ($DSC$)~\cite{sips2009DSC} has been shown to be one of the most performing measures to predict user preferences~\cite{sedlmair2015quality}. These metrics are often supervised, meaning that labels about the instances must be provided in order to assess if the clusters are well separated. 
$DSC$, for instance, computes the number of instances that are closest to the centroid of another class label then their own. More formally,
\begin{equation}
DSC = \frac{| \textbf{y}_i \in \textbf{Y} : CD(\textbf{y}_i, centr(c_{clabel(\textbf{y}_i)})) = true |}{n},
\end{equation}
where \textbf{Y} is the set of points in the visualization, $n$ is the total number of points, $centr(c_{clabel(\textbf{y}_i)})$ computes the virtual point that is at the center of all points with the same class label of $\textbf{y}_i)$ and $CD(\cdot, \cdot)$ computes the distance between two points. 

Other popular measures in this category are the average between-within clusters ($ABW$)~\cite{lewis2012ABW}, the hypothesis margin ($HM$)~\cite{gilad2004HM}, the neighborhood hit ($NH$)~\cite{paulovich2008NH} and the Calinski-Harabasz index ($CAL$)~\cite{calinski1974CAL}. All these metrics measure the separability between clusters, albeit differently. $ABW$ measures the average distances between clusters on the average distances within clusters:
\begin{equation}
    \text{ABW} = \frac{avg_{\textbf{y}_i \stackrel{C}{\not\sim} \textbf{y}_j}dist(\textbf{y}_i, \textbf{y}_j)}{avg_{\textbf{y}_i \stackrel{C}{\sim} \textbf{y}_j}dist(\textbf{y}_i, \textbf{y}_j)} \quad \forall \textbf{y}_i, \textbf{y}_j \in \textbf{Y},
\end{equation}
where $\textbf{y}_i \stackrel{C}{\not\sim} \textbf{y}_j$ means that $y_i$ is not in the same cluster as $y_j$ and $\textbf{y}_i \stackrel{C}{\sim} \textbf{y}_j$ means that the two points are in the same cluster. 

$HM$ uses the nearest point from a different cluster (nearmiss) and the nearest point from the same cluster (nearhit) to define the notions of inter and intra cluster distances:
\begin{equation}
    \text{$HM$} = \sum\nolimits_{\textbf{y}_i \in \textbf{Y}}\frac{1}{2}(\text{dist}(\textbf{y}_i,  \text{nearmiss}(\textbf{y}_i)) - \text{dist}(\textbf{y}_i, \text{nearhit}(\textbf{y}_i))).
\end{equation}

$NH$ makes use of a k-nearest neighbor (kNN) classifier to identify if the points in the visualization are close to their centroid (virtual central point of a cluster). $NH$ corresponds to the accuracy of the classifier.

Finally, $CAL$ is a more complicated measure of the same concepts:
\begin{equation}
    \text{$CAL$} = \frac{\text{BG}}{(k-1)} / \frac{\text{WG}}{(n-k)} = (\bar{d}^2 + \frac{(n-k)}{(k-1)}A_k) / (\bar{d}^2 - A_k),
\end{equation}
where BG (resp. WG) means between groups (resp. within groups). WG is defined by
\begin{equation}
    \text{WG} = \frac{1}{2}\sum_{C_k} (n_{C_k} - 1) \bar{d}^2_{C_k},
\end{equation}
where $C_k$ is $k^{th}$ class label and ${d}^2_{C_k}$ is the squared distances of points belonging to the class ${C_k}$. BG is defined by
\begin{equation}
    \text{BG} = \frac{1}{2}((k-1)\bar{d}^2 + (n-k)A_k),
\end{equation}
where $\bar{d}^2$ is the average of the squared distances between all points, and with
\begin{equation}
    A_k = \frac{1}{(n-k)} \sum_{C_k} ((n_{C_k} - 1)(\bar{d}^2 - \bar{d}^2_{C_k})).
\end{equation}
$A_k$ is simply ``a weighted mean of the differences between the general and the within-group mean squared distances''~\cite{calinski1974CAL}.

%\subsection{Qualitative Results}
%\begin{figure*}[h!]
%    \centering
%    \begin{subfigure}[c]{0.45\linewidth}
%        \includegraphics[width=\linewidth]{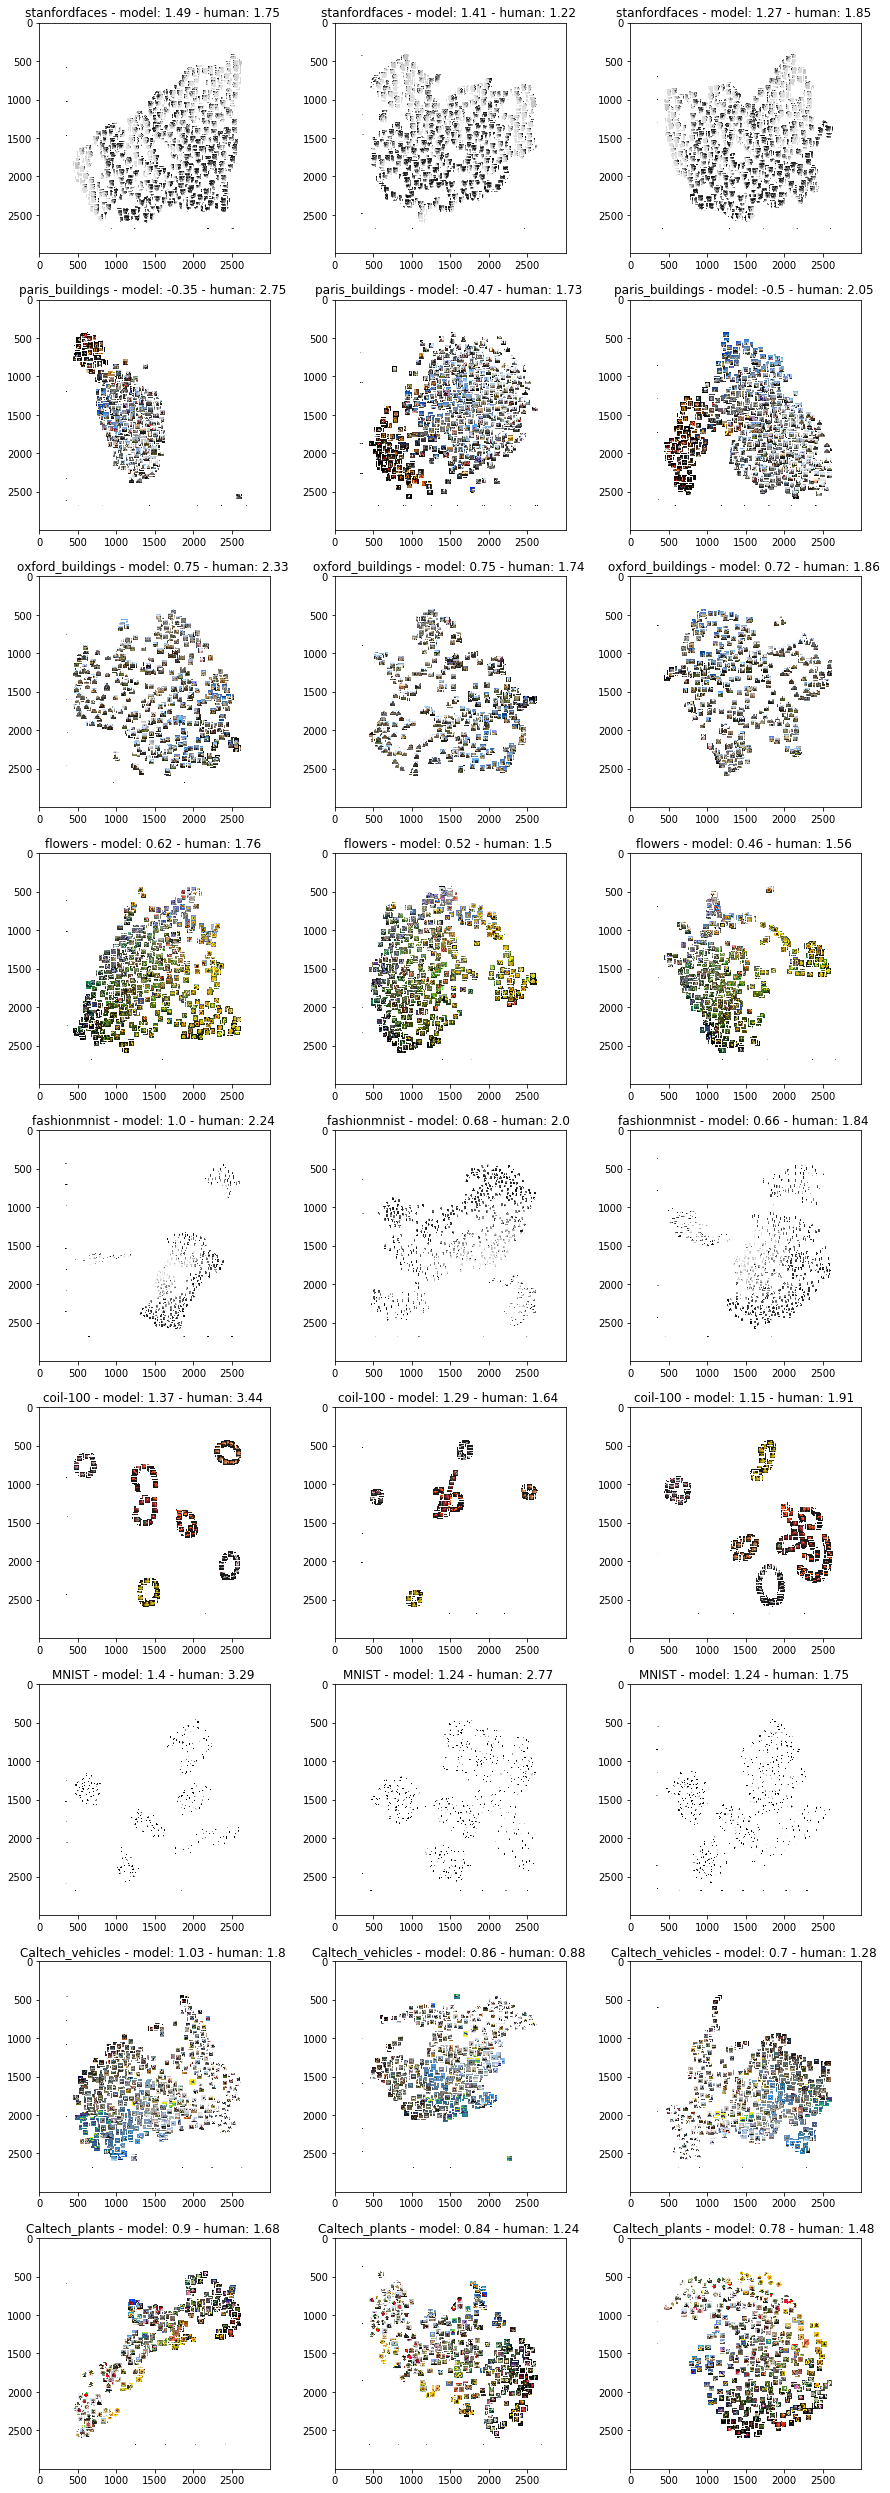}
%        \subcaption{Top 3 projections as selected by the ranked model in experiment 3.}
%    \end{subfigure}
%    ~
%    \begin{subfigure}[c]{0.45\linewidth}
%        \includegraphics[width=\linewidth]{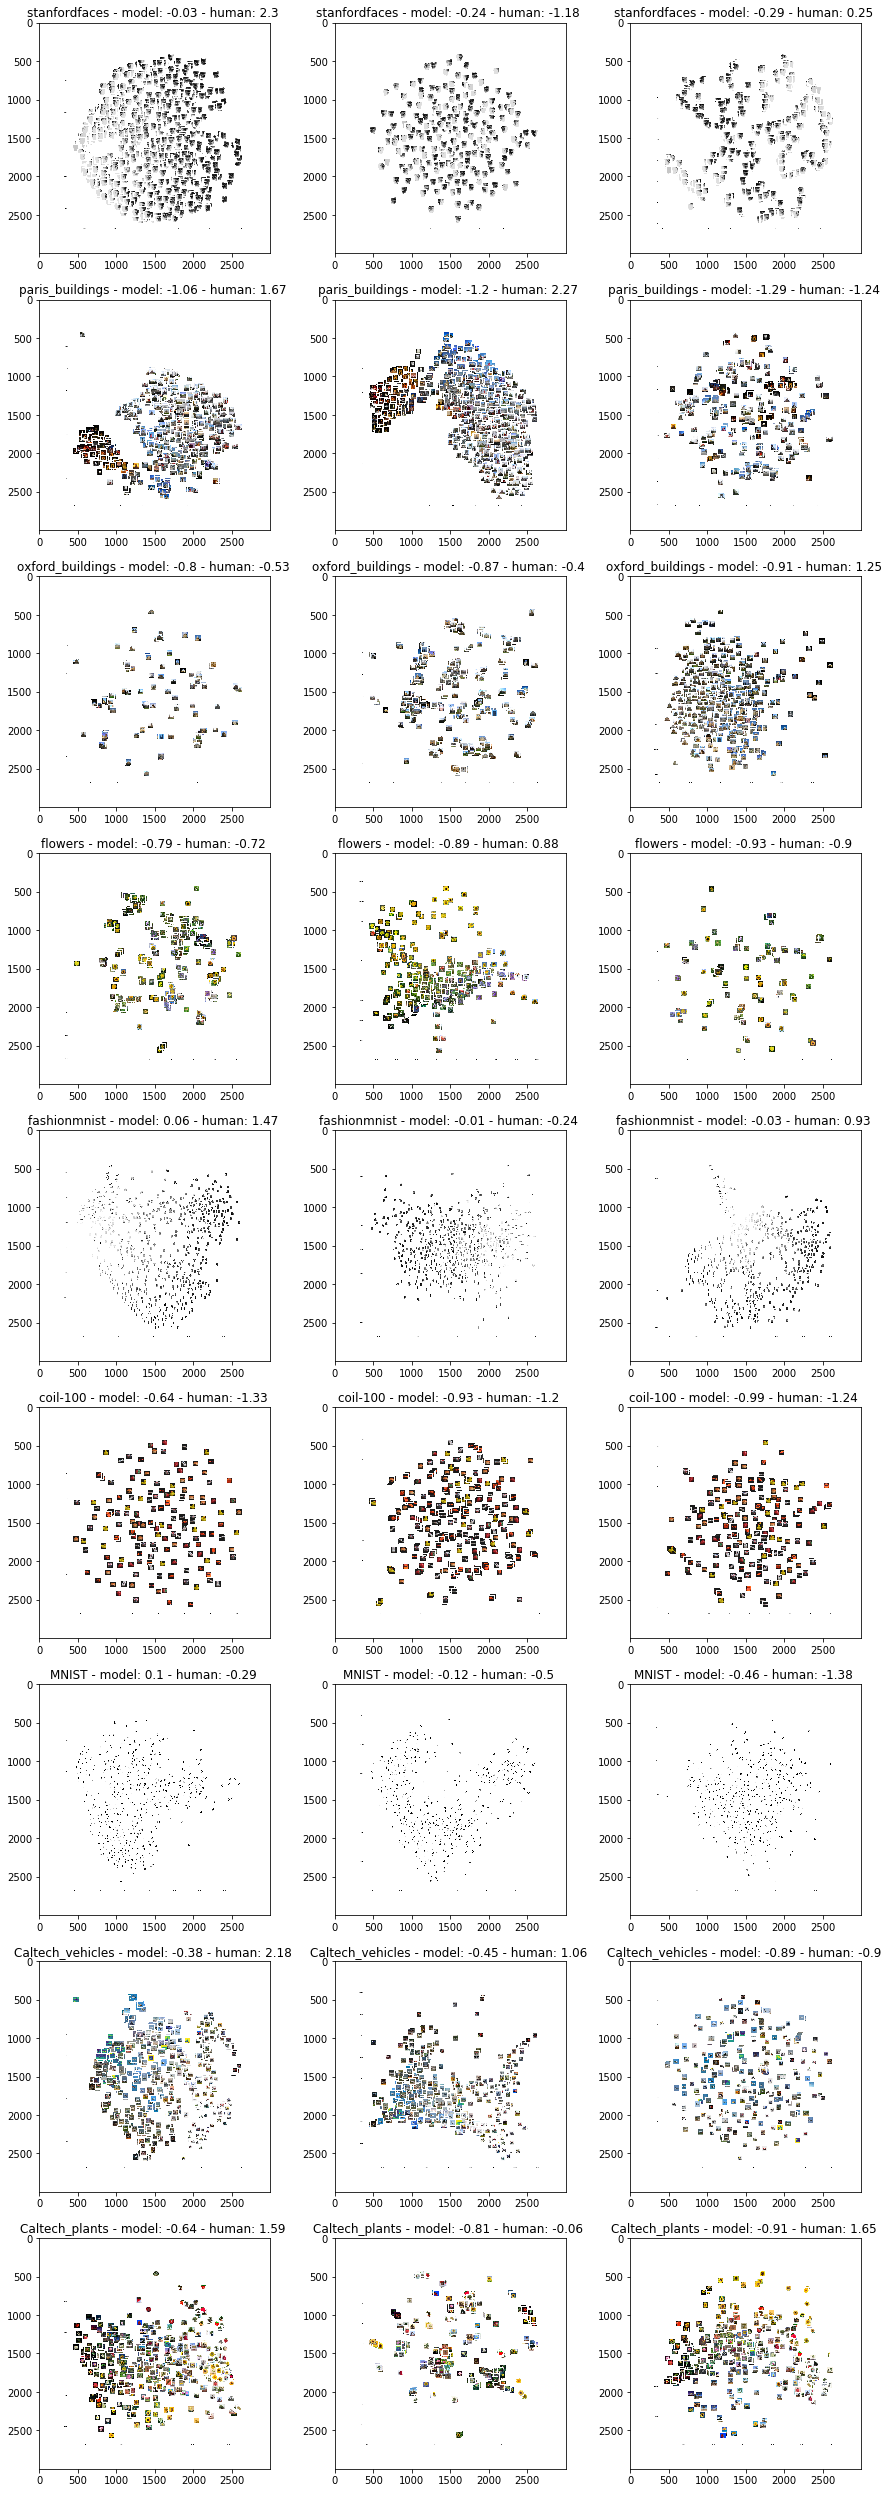}
%        \subcaption{Bottom 3 projections as selected by the ranked model in experiment 3.}
%    \end{subfigure}
%    \caption{Qualitative results of the top 3 and bottom 3 projections for each dataset involved in our analysis.}
%    \label{fig:trial3}
%\end{figure*}
